# Supplementary material for: Probing the Bose-Glass--Superfluid Transition using Quantum Quenches of Disorder
Source: arXiv:1502.02333 ancillary file (2015-02-09)
Supplement: Supplementary file 1 [file SM.pdf]

# Supplemental Material for "Probing the Bose-Glass–Superfluid Transition using Quantum Quenches of Disorder"

C. Meldgin,[1] U. Ray,[1] P. Russ,[1] D. Ceperley,[1] and B. DeMarco[1*]

[1]University of Illinois at Urbana-Champaign,
1110 W Green St, Urbana, IL 61801, USA
*To whom correspondence should be addressed; E-mail: bdemarco@illinois.edu.

February 8, 2015

# 1 Methods and Materials

## 1.1 Experimental Details

Detailed information about the apparatus can be found in Refs. (*1*) and (*2*). The geometric mean of the trap frequencies without the lattice is $\omega = 2\pi\,(53 \pm 3)$ Hz. The lattice potential is ramped on in 100 ms using an exponential function with a 200 ms time constant. For $s$ =10–12 $E_R$, the extra confinement from the gaussian profile of the lattice beams increases the geometric mean trap frequency to approximately $\omega = 2\pi\,(69 \pm 4)$ Hz. The waist of the speckle beam envelope is $161 \pm 2$ $\mu$m, with radial and axial speckle autocorrelation lengths 570 nm and 3 $\mu$m, respectively. The projections of the autocorrelation lengths onto the lattice directions are 650 nm and 790 nm, which are comparable to the 406 nm lattice spacing.

Before time-of-flight imaging, the lattice is band mapped in 300 $\mu$s in order to improve the imaging signal-to-noise ratio (*2*). The gas is supported against gravity by a magnetic field gradient during the 50 ms expansion time.

## 1.2 Quench Time

The time variation of the spatially inhomogeneous disorder potential during the quench can excite excitations such as phonons, for example, by exceeding the local superfluid speed of sound (*3*). To avoid complications from this type of effect, we determine the associated timescale using a simulation of the three-dimensional time-dependent Gross-Pitaevskii equation (*4*). We simulate a disorder quench as in the experiment followed by 20 ms of free expansion. Because it is too computationally intensive to include the lattice, we simulate a trapped gas with the interaction strength adjusted to match the lattice system while coarse graining over the lattice length scales (*5*).

Density distributions from these simulations were column integrated and analyzed using the $\tilde{\chi}^2$ measure of excitation, as with the experimental data. Results for $\Delta = 1\ E_R$, the chemical potential determined by $\mu = m\omega r_i^2/2 + U\langle n_i\rangle/d^3$ (with $U$ for $s = 10\ E_R$), and a trap frequency set to match the experiment are shown in Fig. 1. An exponential fit yields a time constant of $9 \pm 2$ ms. We therefore choose a quench time of 30 ms to suppress excitations that arise only from the time variation of the speckle potential. For $\tau_q = 30$ ms, the simulated $\tilde{\chi}^2$ is approximately 20 times smaller than in the experiment for similar $\Delta$.

## 1.3 SF–BG Transition Dynamics

The exploration of the dynamical timescale of the SF–BG transition is carried out using a procedure alternative to that for the $\tilde{\chi}^2$ measurement. We measure condensate fraction using TOF imaging at the end of a slow turn-off of the lattice over 60 ms and 150 ms thermalization time in the trap (Fig. 2). Condensate fraction is inverted to temperature $T$ using a semi-ideal model (*6*).

## 1.4 QMC Simulations

The simulations were performed using Stochastic Series Expansion algorithm, which is statistically exact for the systems considered here (*7*). All parameters for the DBHM were generated using the Löwdin orthonormalization method discussed in Ref. (*8*). For the large systems we consider here, a specialized iterative procedure based on Iannazzo iteration is needed to compute the inverse square

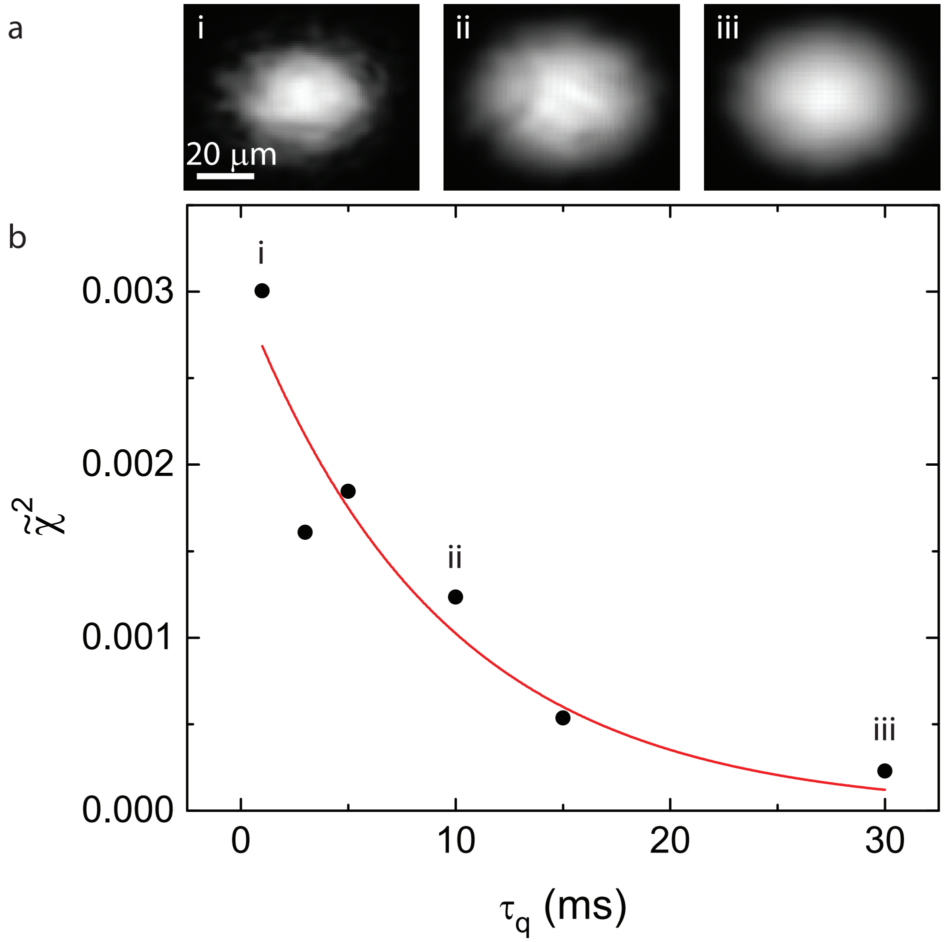


Figure 1: Time-dependent Gross Pitaevskii simulations including 20 ms of free expansion following the quench for different quench times $\tau_q$. (a) Simulated column density profiles for $\tau_q = 1$ (i), 10 (ii), and 30 ms (iii). (b) Excitation strength $\tilde{\chi}^2$ as $\tau_q$ is varied. The solid line is a fit to an exponential decay.

root of the overlap matrix (*9*). We use this procedure to coarse grain the experimental potential as closely as possible while preserving all its statistical properties.

Detecting the SF–BG phase transition in trap-free geometries, with periodic boundary conditions, is possible via the winding number formulation used to calculate the superfluid fraction (*10*). In such cases a BG is signaled by the absence of net winding paths across the boundary of the simulation cell. The superfluid fraction measures the coherence properties of the system that manifest as long loops wound throughout the system. At ultra-low temperature, the dominant contribution to the density matrix is from the ground state, and the winding captures its non-local or spatially

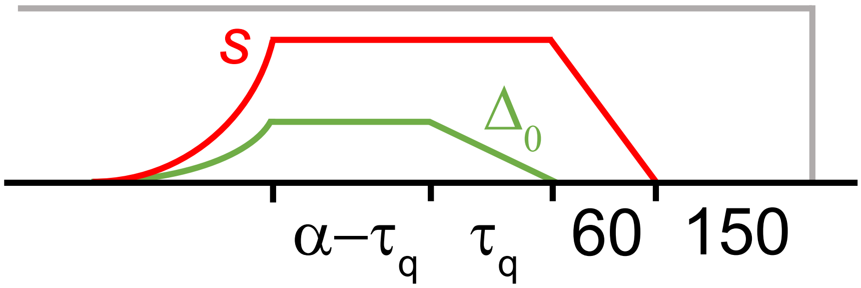


Figure 2: Timing used for dynamics measurement. The lattice potential (red) is on for a fixed time $\alpha$, and the quench time $\tau_q$ of the disorder potential (green) is varied. After the quench, the lattice is ramped off in 60 ms, and the atoms are allowed to thermalize in the trap (gray) for 150 ms. For the data shown in Fig. 4 in the main text, $\alpha$=45 ms for $\Delta = 0.35\ E_R$, and $\alpha$=150 ms for $\Delta = 1\ E_R$.

extended nature. This extended property is also visible in the single particle eigenstates that can be measured from the single particle density matrix ($\rho_1 \equiv \langle \hat{b}_i^\dagger \hat{b}_j \rangle$). Global coherence manifests itself by the macroscopic occupation of a single particle mode, known as Bose-Einstein condensation (*11, 12*).

There is a technical point to be made about Bose-Einstein condensation and superfluidity. The latter is a much more general phenomena that can arise even in the absence of true long range order, for instance in the 2D Berninski-Kosterlitz-Thouless (BKT) transition which occurs via the unbinding of topological vortex defects (*13*). Physically it measures how the system responds to rotations, i.e., it is a flow property. Condensation, on the other hand, requires long-range order (*12*). The dramatic difference between these two measures is illustrated in the context of strongly interacting $^4He$ in 3D, where systems are only 10% condensed due to depletion, but are 100% superfluid (*10*). In either case, whether by algebraic decay of the correlation length or decay of correlations asymptotically to a non-zero value at large separations, the presence of global coherence inevitably points to the existence of an extended single particle ground state.

The trap complicates affairs considerably as, strictly speaking, extended states are not possible. Concurrently, measuring the superfluid fraction via the global winding number is also no longer possible. Furthermore, trapped systems exhibit multiple domains and distinguishing between them requires alternative local observables. The local measure of superfluidity is given by $\rho_s(r) =$

$2\pi^2\langle AA(r)\rangle/\beta$, where $A(r) = 1/2\sum_{ik} r_k^i \times r_{k+1}^i$ is the total area of paths subtended in imaginary time by all particles. It measures the coherence of a local region due to rotations about some chosen axis (*14*). Additionally, on diagonalizing $\rho_1$ we obtain the eigenpairs $(\psi_i(r), N_i)$ corresponding to the eigenstate and the occupation number of single particle modes (*15*). These can be used to construct the single particle density distributions $n_i(r) \equiv N_i|\psi_i(r)|^2$, with $n_0(r)$ corresponding to the condensate density. In principle all eigenstates can be calculated, but in general QMC data is noisy and only the first few largest eigenvalues and the corresponding eigenstates can be obtained using practical run times.

As discussed in the main text, for these systems, we do not observe any fragmentation with multiple macroscopic condensates. Instead, we find that the system falls into two distinct behaviors. The first type of behavior corresponds to $\Delta < \Delta_{th}$, where there is one distinct macroscopic condensate (with $\sim O(N)$ occupation) and all subsequent eigenstates have small occupation ($\ll O(N)$). In this region the macroscopic condensate extends throughout the system. We find that the first few ($\sim 10$) largest eigenstates are also extended and spatially coincidental with the macroscopic condensate. Such eigenstates represent the depleted modes that arise due to interactions or thermal excitations (the latter is suppressed at ultra-low temperature). $\rho_s(r)$ measured in this regime (relative to and averaged over the axes $x = 0$, $y = 0$ and $z = 0$) shows the presence of a global superfluid spatially coincidental with the condensate.

For $\Delta \geq \Delta_{th}$, a new type of behavior arises. The condensate starts shrinking and there are regions in the gas that do not participate in it. Additionally $\rho_s(r)$ indicates that such regions are devoid of any superfluid. Thus, we can account for atoms in this region as part of the BG domain that develops. For practical purposes such regions are composed of sites with $n_0(r) < n_{th}$, where $n_{th}$ is a small threshold parameter. Over the range of QMC data we find that using $n_{th} = 10^{-5}$ is ideal for all measurements. We have checked that the phase boundary value $\Delta_{th}$ that we extract is not sensitive to $n_{th}$.

The BG domain that we identify in this manner consists of SF puddles that nonetheless remain localized and globally incoherent. An example of this spectacular localization transition is shown

in the insets in Fig. 2b in the main text. The single particle eigenstates for trapped systems consist of the macroscopically occupied condensate, associated extended depleted modes, and localized single particle states spatially coincidental with the BG domain. The occupation number of localized SF puddles in the BG domain rapidly increases as the SF–BG threshold is crossed. It must ultimately decrease as more incoherent puddles are formed due to increase in disorder. The occupation numbers of these localized modes remain non-macroscopic ($\ll O(N)$).

## 1.5 Temperature

The QMC simulations are carried out in the ultra-low temperature regime, corresponding to $k_B T = t$. In contrast, the experiments access low but non-zero temperature. Understanding the impact of non-zero temperature on the quench measurement is complicated by the problem of precisely determining temperature in optical lattice experiments (*16*). We therefore use a standard technique to estimate temperature in the lattice by assuming the entropy per particle $S/N$ inferred from TOF measurements of condensate fraction in the trap is preserved during the lattice turn-on. QMC simulations are then applied to convert $S/N$ to temperature in the disordered lattice. We consider the highest interaction and disorder strengths we access in this work ($s = 12$ and $\Delta = 1\ E_R$), where the maximal impact of non-zero temperature is expected.

The temperature is sufficiently low in the experiment so that we can only determine an upper bound on $S/N$. Based on an analysis of the imaging noise and images taken at short and long expansion times (i.e., low and high optical depth), we estimate that the condensate fraction before turning on the lattice is greater than 0.9. This lower limit implies on upper bound of 0.4 $k_B$ per particle on $S/N$, according to a semi-ideal model (*6*). We therefore estimate that 0.4 $k_B > S/N > 0\ k_B$ for the measurements presented in this work.

We compare this entropy estimate from the experiment to the results of QMC simulations. Using the energy per particle ($E/N$) from QMC runs, we infer the entropy per particle as a function of temperature. The results shown in Fig. 3a were obtained by fitting $E/N$ to a cubic spline for the sampled points. The ultra-low temperature behavior is obtained by fitting the low temperature

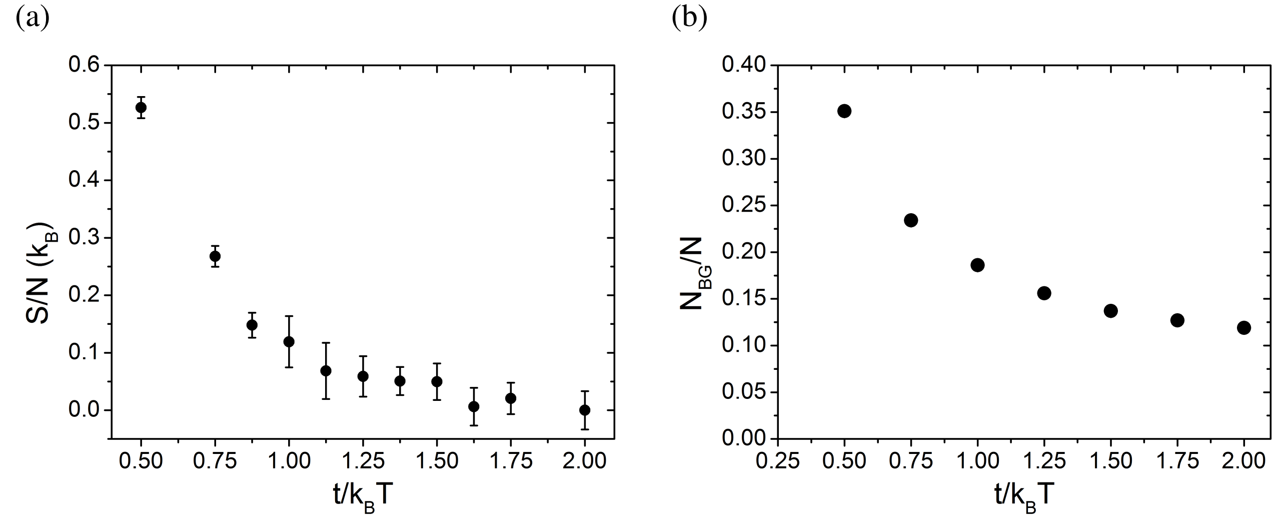


Figure 3: (a) The entropy per particle estimated from the energy per particle using QMC simulations. (b) The dependence of the Bose-glass fraction on temperature for $s = 12\ E_R$ and $\Delta = 1\ E_R$. The cross-over behavior and the saturation of the BG fraction as $T \to 0$ are apparent.

points to a exponential function. The entropy per particle $S/N$ is then obtained from $E/N$ via integration. This procedure is similar to those used for clean systems (*17*).

Given the bounds from the experiment, we estimate that $T < 1.4t/k_B$ for $s = 12$ and $\Delta = 1\ E_R$. A method for understanding how this non-zero $T$ affects the quench measurements and determination of $\Delta_{th}$ is unavailable and beyond the scope of this work. To gauge the impact of non-zero $T$, we use equilibrium QMC simulations to calculate how $N_{bg}/N$ changes with temperature. Fig. 3b shows results for $s = 12$ and $\Delta = 1\ E_R$. The regime sampled by the experiment is close to the $T \to 0$ limit and is not dominated by thermal excitation. We conclude an insulating domain persists in the zero-temperature limit, and the localized states that arise in the BG domain are robust in the temperature regime sampled in the experiment.

## 1.6 Disorder Averaging

Experimentally, a systematic accounting of disorder averaging is intractable. However, over the course of experiments, there are small shifts in the focal point of the speckle light used to generate the disorder potential. In the presence of such shifts, we find no observable changes in the qualitative or quantitative behavior of the gas. Theoretically, disorder averaging is also extremely

challenging for these large systems ($60^3$ lattice points with $27,000$ particles; c.f. (*18*) with lattices of size $8^3$–$16^3$ at unit filling for box-disorder systems). We are able to obtain a systematic sense of the uncertainty that results from using different disorder realizations by running simulations for $10$ uncorrelated disorder potentials at $\Delta = 1\ E_R$ and $s = 12\ E_R$. We expect these parameters, which correspond to the strongest interactions and disorder we have considered, to exhibit the largest possible deviations. We find that disorder averaging introduces an uncertainty of $\sim 7\%$ to $N_{bg}/N$ under these conditions.

# References


1. M. Pasienski, D. McKay, M. White, B. DeMarco, *Nat. Phys.* **6**, 677 (2010).
2. D. McKay, M. White, B. DeMarco, *Phys. Rev. A* **79**, 063605 (2009).
3. C. Pethick, H. Smith, *Bose-Einstein condensation in dilute gases* (Cambridge University Press, 2002).
4. W. Bao, S. Jin, P. Markowich, *Siam J. Sci. Comput.* **25**, 27 (2003).
5. M. Greiner, Ultracold quantum gases in three-dimensional optical lattice potentials, Ph.D. thesis, Ludwig-Maximilians-Universität München (2003).
6. M. Naraschewski, D. M. Stamper-Kurn, *Phys. Rev. A* **58**, 2423 (1998).
7. A. W. Sandvik, *Phys. Rev. B* **59**, R14157 (1999).
8. S. Q. Zhou, D. M. Ceperley, *Phys. Rev. A* **81**, 013402 (2010).
9. N. J. Higham, *Functions of Matrices: Theory and Computation* (Society for Industrial and Applied Mathematics, Philadelphia, PA, USA, 2008).
10. D. M. Ceperley, *Rev. Mod. Phys.* **67**, 279 (1995).
11. O. Penrose, L. Onsager, *Phys. Rev.* **104**, 576 (1956).

12. A. J. Leggett, *Quantum liquids: Bose condensation and Cooper pairing in condensed-matter systems* (Oxford University Press, 2006).

13. N. Goldenfeld, *Lectures on Phase Transitions and the Renormalization Group*, Frontiers in physics (Addison-Wesley, Advanced Book Program, 1992).

14. Y. Kwon, F. Paesani, K. B. Whaley, *Phys. Rev. B* **74**, 174522 (2006).

15. U. Ray, D. M. Ceperley, *Phys. Rev. A* **87**, 051603 (2013).

16. D. C. McKay, B. DeMarco **74**, 054401 (2011).

17. D. McKay, *et al.*, *arXiv: 1411.5593* (2014).

18. L. Pollet, N. Prokof'ev, B. Svistunov, M. Troyer, *Phys. Rev. Lett.* **103**, 140402 (2009).
